# Supplementary material for: Evidence of electronic states driving current-induced insulator-to-metal transition
Source: arXiv:2504.17871 source file (2025-04-24)

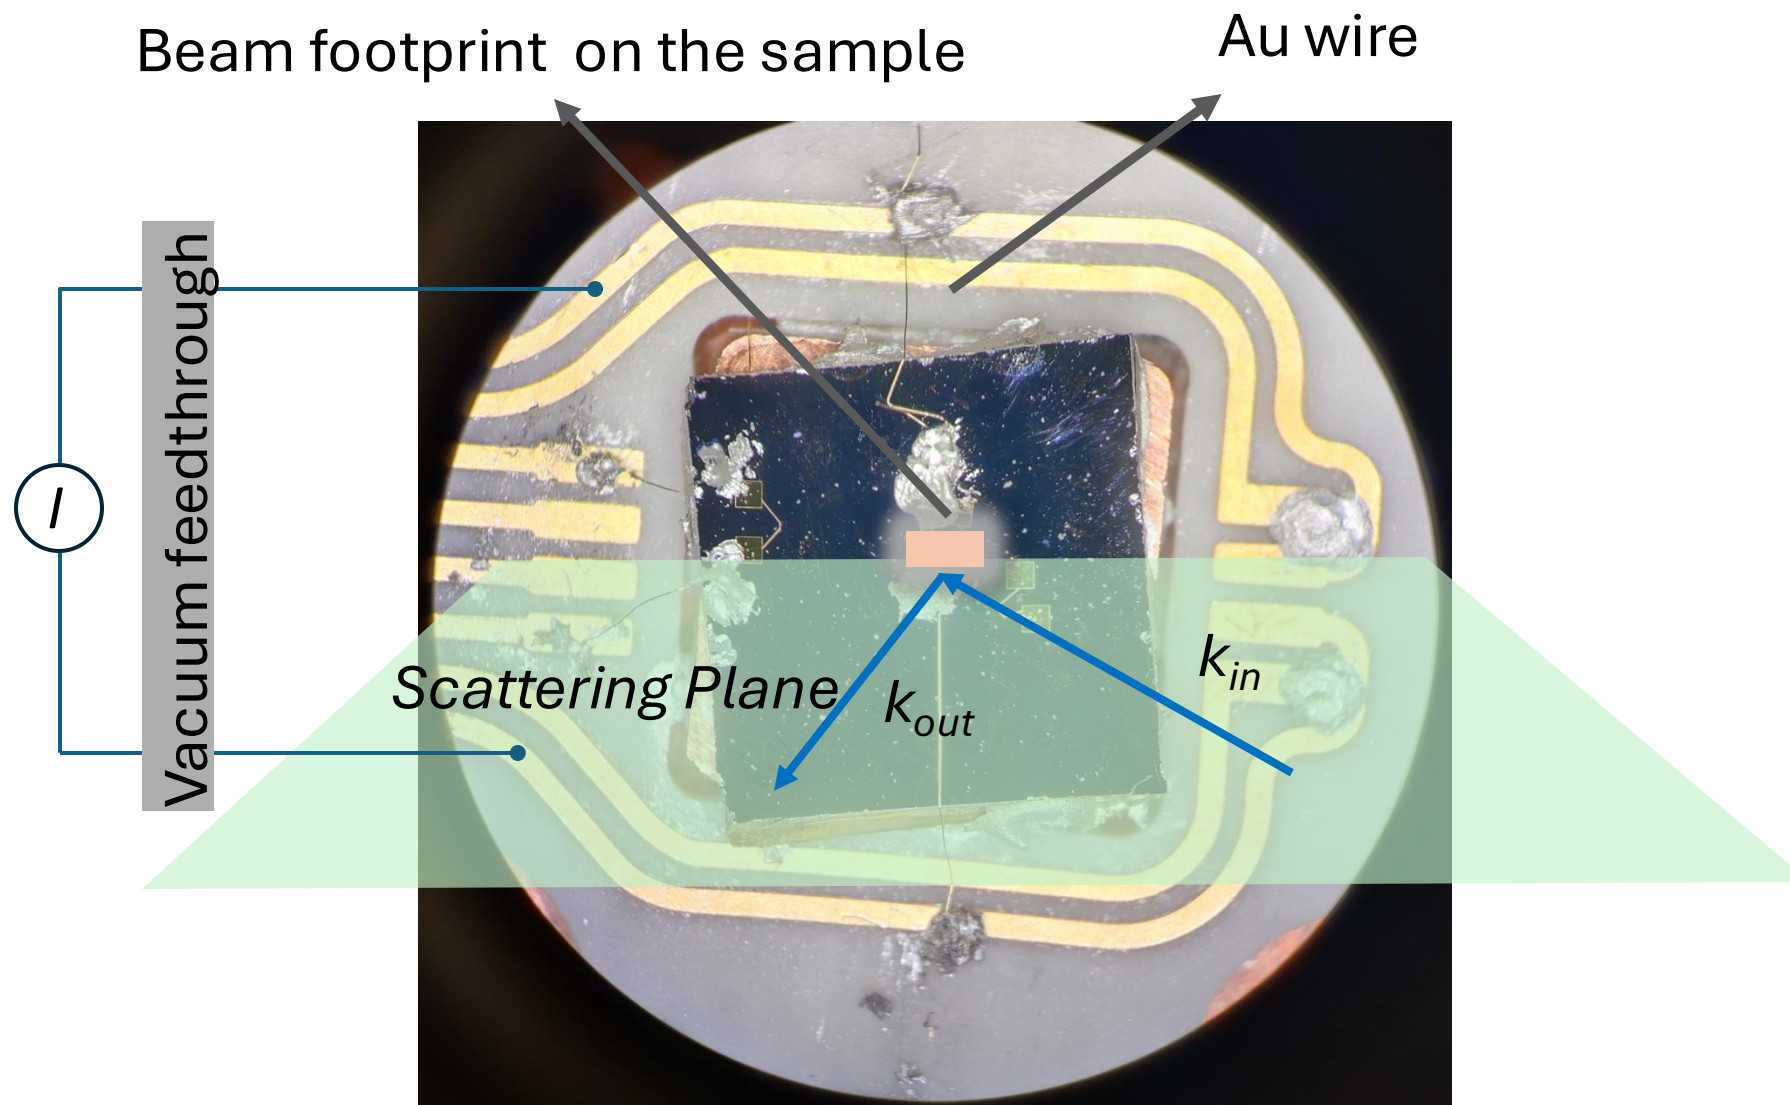

Supplement: Supplementary file 1 [file supp_drawings_v2.pdf]
